# Supplementary material for: Attention Hijackers: Detect and Disentangle Attention Hijacking in LVLMs for Hallucination Mitigation
Source: arXiv:2503.08216 source file (2025-03-14)
Supplement: Supplementary file 1 [file X_suppl.tex]

\clearpage
% \setcounter{page}{1}
% \maketitlesupplementary
\begin{appendices}

\onecolumn

\begin{center}{\bf \Large Attention Hijackers: Detect and Disentangle Attention Hijacking in LVLMs for Hallucination Mitigation}\end{center}
\begin{center}{\Large Appendix}\end{center}

% 
% Having the supplementary compiled together with the main paper means that:
% 
% \begin{itemize}
% \item The supplementary can back-reference sections of the main paper, for example, we can refer to \cref{sec:intro};
% \item The main paper can forward reference sub-sections within the supplementary explicitly (e.g. referring to a particular experiment); 
% \item When submitted to arXiv, the supplementary will already included at the end of the paper.
% \end{itemize}
% % 
% To split the supplementary pages from the main paper, you can use \href{https://support.apple.com/en-ca/guide/preview/prvw11793/mac#:~:text=Delete%20a%20page%20from%20a,or%20choose%20Edit%20%3E%20Delete).}{Preview (on macOS)}, \href{https://www.adobe.com/acrobat/how-to/delete-pages-from-pdf.html#:~:text=Choose%20%E2%80%9CTools%E2%80%9D%20%3E%20%E2%80%9COrganize,or%20pages%20from%20the%20file.}{Adobe Acrobat} (on all OSs), as well as \href{https://superuser.com/questions/517986/is-it-possible-to-delete-some-pages-of-a-pdf-document}{command line tools}.

% \section{Theoretical Analysis of Attention Hijacking}
% \label{sec:Theoretical_Analysis}

\begin{figure}[h]
    \centering
    \includegraphics[width=0.7\linewidth]{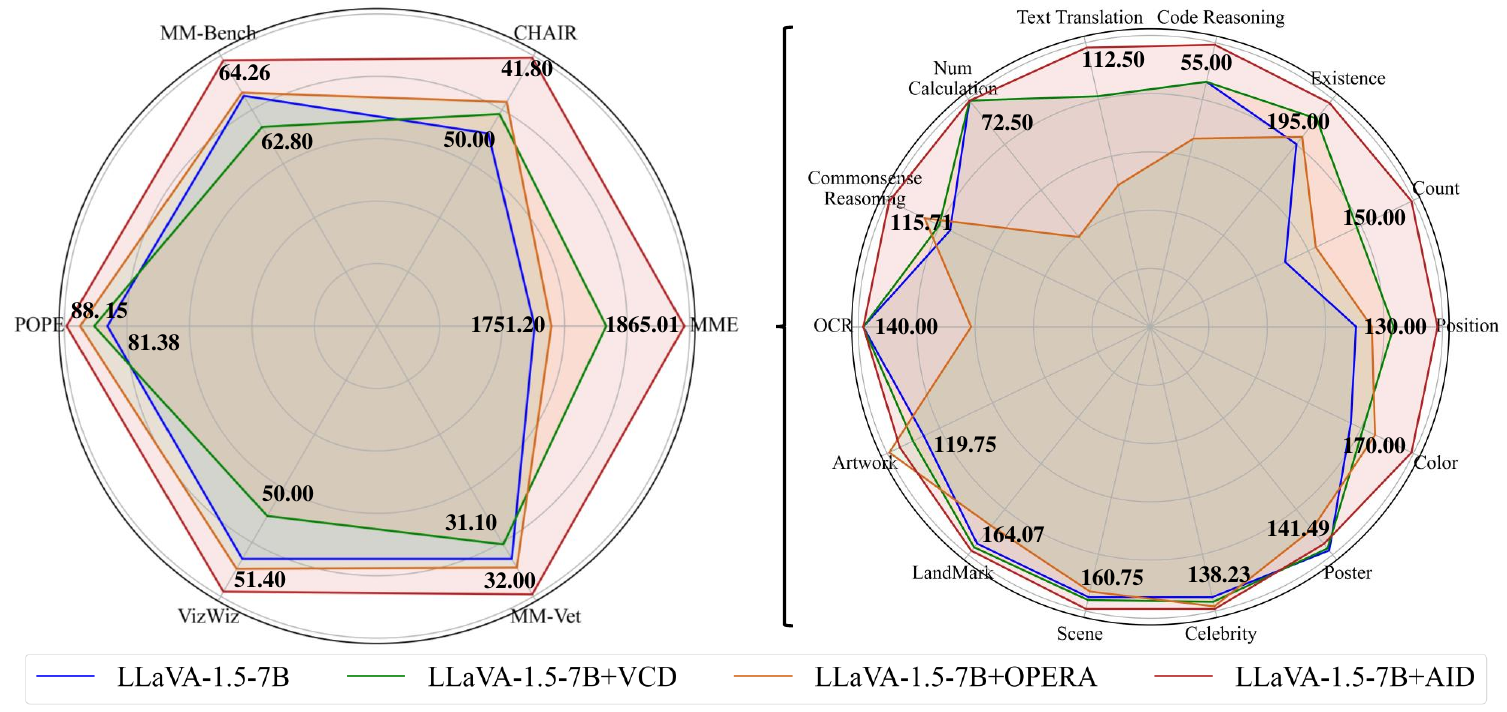}
    \caption{AID demonstrates strong performance across seven benchmarks spanning various domains (Left), with particularly outstanding results on the MME benchmark (Right).}
    \label{fig:hexagon}
\end{figure}

% \hypersetup{linkcolor=black}
% \etocdepthtag.toc{mtappendix}
% \etocsettagdepth{mtchapter}{none}
% \etocsettagdepth{mtappendix}{subsection}
% \tableofcontents
% \hypersetup{linkcolor=red}

{
\hypersetup{
    linkcolor=black
}
{\centering
 \begin{minipage}{\textwidth}
 \let\mtcontentsname\contentsname
 \renewcommand\contentsname{\MakeUppercase\mtcontentsname}
 \noindent
 \rule{\textwidth}{1.4pt}\\[-0.75em]
 \noindent
 \rule{\textwidth}{0.4pt}
 \tableofcontents
 \rule{\textwidth}{0.4pt}\\[-0.70em]
 \noindent
 \rule{\textwidth}{1.4pt}
 % \setlength{\cftfigindent}{0pt}
 % \setlength{\cfttabindent}{0pt}
%  \listoftables
%  \listoffigures
 \end{minipage}\par}
}
% \resumetocwriting
\clearpage

\section{Additional Experiments, Results, and Discussions}
\label{sec:additional_experiments}

In this appendix, we present further information on the benchmarks mentioned in the main paper.
% We use the following five benchmarks to assess hallucinations:

\textbf{Offline Polling based Object Probing Evaluation (POPE)}~\cite{chen2024halc} Following HALC~\cite{chen2024halc}, we utilize offline POPE (OPOPE) benchmark with both accuracy and F1-score as evaluation metrics to assess VH. 
As shown in Tables~\ref{tab:opope-appendix}, we observe several key findings:
(1) AID consistently achieves optimal performance across most experimental settings, surpassing both state-of-the-art methods.
(2) AID demonstrates consistent VH mitigation capabilities across three distinct LVLM architectures, highlighting its versatility and plug-and-play nature. This architectural agnosticism suggests broad applicability across different model frameworks.
    
    \begin{table*}[htbp]
          \centering
          \begin{tabular}{c|c|cccccc}
            \toprule
            \multirow{2}[2]{*}{} & \multirow{2}[2]{*}{Methods}  
                      & \multicolumn{2}{c}{Random} & \multicolumn{2}{c}{Popular} & \multicolumn{2}{c}{Adversarial} \\
                  &       & Accuracy & F1 score & Accuracy & F1 score & Accuracy & F1 score \\
            \midrule
            \multirow{6}[2]{*}{LLaVA-1.5} & Greedy & 79.25  & 81.75  & 74.50  & 78.48  & 71.50  & 76.54    \\
                  & Beam Search                    & 83.75  & 84.84  & 82.50  & 83.87  & 79.50  & 81.61  \\
                                           & OPERA & 79.75  & 82.03  & 79.00  & 81.49  & 76.50  & 79.74   \\
                                           & VCD   & 76.75  & 80.24  & 70.25  & 76.05  & 70.25  & 75.95   \\
                                           & DoLa  & 82.00  & 83.56  & 81.75  & 83.37  & 78.50  & 80.97   \\
                  % & SID   & 77.93  & 72.84  & 74.89  & 69.34  & 72.77  & 68.30  \\
                  % & HALC  & 77.08  & 72.16  & 74.15  & 69.09  & 72.46  & 68.04  \\
                  \rowcolor{aliceblue}     & Ours  & \textbf{90.25} & \textbf{90.12}  & \textbf{88.75 } & \textbf{88.77} & \textbf{85.00} & \textbf{85.57}  \\
            \midrule
            \multirow{6}[2]{*}{MiniGPT4} & Greedy & 57.50 & 69.96 & 51.00 & 66.77 & 53.50 & 67.93 \\
                                    & Beam Search & 57.50 & 69.64 & 52.00 & 67.01 & 54.75 & 68.30 \\
                                          & OPERA & 57.25 & 69.62 & 52.25 & 67.23 & 54.50 & 68.29  \\
                                          & VCD   & 61.50 & 68.82 & 60.25 & 66.80 & 58.50 & 66.26 \\
                                          & DoLa  & 57.50 & 69.85 & 53.25 & 67.70 & 55.25 & 68.65  \\
                  % & SID   & 69.05  & 56.53  & 65.58  & 53.53  & 65.45  & 53.52  \\
                  % & HALC  & 69.13  & 56.86  & 65.62  & 53.63  & 65.73  & 53.69  \\
                 \rowcolor{aliceblue} & Ours  & \textbf{70.50} & \textbf{75.41} & \textbf{61.25} & \textbf{70.01} & \textbf{61.75} & \textbf{70.29} \\
            \midrule
            \multirow{6}[2]{*}{ mPLUG-Owl2} & Greedy & 79.00 & 82.22 & 76.50 & 89.49 & 73.50 & 78.54   \\
                              & Beam Search          & 85.75 & 86.83 & 82.00 & 83.92 & 79.00 & 81.73 \\
                              & OPERA                & 86.25 & 87.29 & 80.00 & 82.53 & 76.75 & 80.25   \\
                              & VCD                  & 77.00 & 80.50 & 74.00 & 78.51 & 74.25 & 78.67  \\
                              & DoLa                 & 87.25 & 88.11 & 83.00 & 84.75 & 79.50 & 82.17 \\
                  % & SID   & 75.72  & 69.31  & 71.79  & 81.90  & 69.12  & 64.10  \\
                  % & HALC  & 75.62  & 69.04  & 70.24  & 82.40  & 68.35  & 63.51  \\
                  \rowcolor{aliceblue} & Ours  & \textbf{90.25}  & \textbf{90.81}  & \textbf{86.00}  & \textbf{86.72}  & \textbf{83.25 } & \textbf{84.52 } \\
            \bottomrule
            \end{tabular}%
          \caption{Comparison of the average Accuracy and F1-score evaluation results under different settings (i.e., \textit{ Random, Popular, Adversarial}) with different baselines and our AID on offline POPE benchmark~\cite{li2023evaluating, chen2024halc} of five random runs. Higher F1-score indicate better performance and bold indicates the best results. }
          \label{tab:opope-appendix}%
        \end{table*}%

\textbf{CHAIR}~\cite{rohrbach2018_chair} evaluates how well the generated captions align with the content of the given image. 
CHAIR consists of two versions: CHAIR\_S, which measures the inaccuracies at the sentence level, and CHAIR\_I, which evaluates at the object level within the sentence by comparing the number of false objects to the total number of objects. 
For evaluation, we use the val2014 split of the MSCOCO~\cite{lin2014microsoft} dataset, which includes annotations for 80 object categories. 
We randomly select 500 images from the entire dataset and used the prompt ``Please describe this image in detail.'' for the LVLM.

\begin{table*}[h!]
\centering
\small
\resizebox{0.5 \linewidth}{!}{
\begin{tabular}{llll}
\toprule
\multirow{2}{*}[-0.5ex]{\textbf{Method}} & \multicolumn{3}{c}{\quad\textbf{CHAIRs}}  \\
\cmidrule{2-4}				
 & \bf CHAIRs\down & \bf CHAIRi\down   & \bf Length \\
\midrule
 LLaVA1.5-7B                            & 50.00         \basex{0.0}  & 15.40           \basex{0.0}    & 100.6 \basex{0.0} \\
  + VCD~\citep{leng2023mitigating_vcd}  & 48.60         \down{1.4}   & 14.90           \down{0.5}     & 100.4 \down{0.2} \\
  + OPERA~\citep{huang2023opera}        & 47.80         \down{2.2}   & 14.60           \down{0.8}     & 98.60  \down{2.0} \\
  \rowcolor{aliceblue} \textbf{+ AID (Ours)}                 & \textbf{41.80} \down{8.2}   & \textbf{13.00} \down{2.4}     & 96.80   \down{3.8} \\ 
\midrule 
 GLM-4V-9B                              & 40.40 \basex{0.0}         & \textbf{9.00} \basex{0.0}    & 218.20 \basex{0.0} \\
   + VCD~\citep{leng2023mitigating_vcd} & 42.20 \upbad{1.8}         & 9.60 \upbad{0.6} &  239.80 \upbad{21.6} \\
   + OPERA~\citep{huang2023opera}       & - & -  & - \\
    \rowcolor{aliceblue} \textbf{+ AID (Ours)}               & \textbf{38.20} \down{2.2} & \textbf{8.80} \down{0.2} & 210.00 \down{6.2} \\
\midrule
 Qwen-VL-10B                           & 10.20 \basex{0.0}         & 7.20 \basex{0.0}          & 22.50 \basex{0.0} \\
  + VCD~\citep{leng2023mitigating_vcd} & 13.00 \upbad{2.8}        & 12.3 \upbad{5.1}          & 115.7 \upbad{93.2} \\
  + OPERA~\citep{huang2023opera}       & - & -  & - \\
   \rowcolor{aliceblue} \textbf{+ AID (Ours)}               & \textbf{5.200} \down{5.0} & \textbf{3.30} \down{3.9}  & 12.90 \down{9.6} \\
\bottomrule
\end{tabular}}
% \vspace{-5pt}
\caption{Results on CHAIRS dataset. Best-performing method per model size and dataset is highlighted in bold; arrows indicate improvement or degradation over the baseline, where lower values indicate better performance.}
\label{tab:res_chairs}
\end{table*}

\begin{figure*}[h]
    \centering
    \includegraphics[width=1\linewidth]{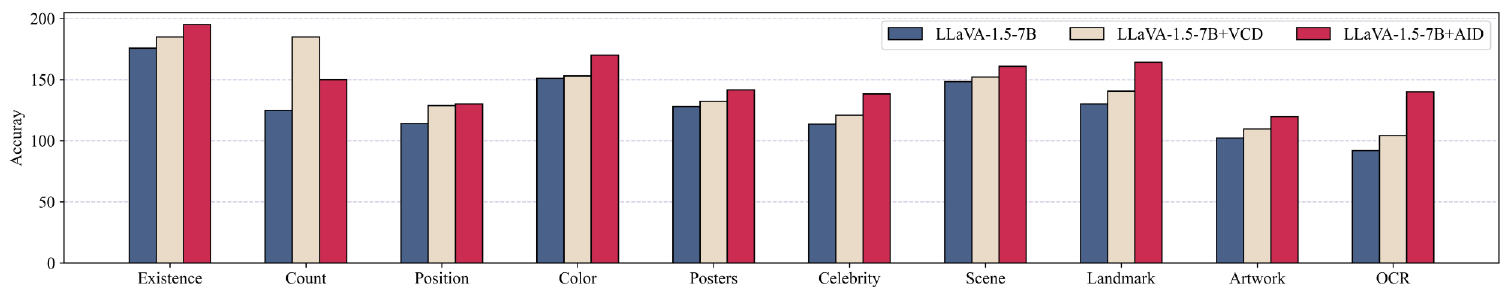}
    \caption{MME full set results on LLaVA-1.5. AID leads to consistent enhancement in LVLMs’ perception capacities while preserving their recognition competencies.}
    \label{fig:res_mme}
\end{figure*}

\textbf{LVLM Evaluation (MME)}~\cite{fu2023mme} evaluates the capabilities of LVLMs, dividing the evaluation into two major categories: perception and cognition. 
The perception category includes fine-grained tasks such as existence, count, location, rough color, poster, celebrity, scene, landmark, artwork identification, and OCR. 
The cognition category includes tasks like commonsense reasoning, numerical calculations, text translation, and code reasoning. 
All questions in this benchmark are structured to be answered with a simple yes or no.

\begin{table*}[h!]
\centering
\small
\resizebox{0.5 \linewidth}{!}{
\begin{tabular}{lllll}
\toprule
\multirow{2}{*}[-0.5ex]{\textbf{Method}} & \multicolumn{3}{c}{\quad\textbf{CHAIRs}}  \\
\cmidrule{2-4}				
 & \bf CHAIRs\down & \bf CHAIRi\down  & \bf Length \\
\midrule
 LLaVA1.5-7B~\citep{liu2023visual_llava} & 50.00         \basex{0.0}  & 15.40           \basex{0.0}    & 100.6 \basex{0.0} \\
  \rowcolor{aliceblue} \textbf{+ AID (Ours)}                  & \textbf{41.80} \down{8.2}   & \textbf{13.00} \down{2.4}    & 96.80   \down{3.8} \\ 
\midrule 
 InstructBLIP~\citep{dai2023instructblip} & 57.2 \basex{0.0}         & \textbf{24.6} \basex{0.0}   & 108.7 \basex{0.0} \\
    \rowcolor{aliceblue} \textbf{+ AID (Ours)}               & \textbf{52.8} \down{4.4} & \textbf{23.4} \down{1.2}  & 109.6 \up{0.9} \\
\midrule
 MiniGPT4~\citep{zhu2023minigpt4}      & 36.6 \basex{0.0}         & 12.8 \basex{0.0}         & 81 \basex{0.0} \\
   \rowcolor{aliceblue} \textbf{+ AID (Ours)}               & \textbf{32.2} \down{4.4} & \textbf{11.7} \down{1.1}  & 77.4 \down{3.6} \\
\bottomrule
\end{tabular}}
% \vspace{-5pt}
\caption{Results on CHAIRS of dataset. Best-performing method per model size and dataset is highlighted in bold; arrows indicate improvement or degradation over the baseline, where lower values indicate better performance.}
\label{tab:res_chairs_5000}
\end{table*}

% \begin{table*}[h!]
% \centering
% \small
% \resizebox{0.7 \linewidth}{!}{
% \begin{tabular}{llllll}
% \toprule
% \multirow{2}{*}[-0.5ex]{\textbf{Method}} & \multicolumn{4}{c}{\quad\quad\textbf{CHAIRs}}  \\
% \cmidrule{2-5}				
%  & \bf CHAIRs & \bf CHAIRi & \bf Recall & \bf Len \\
% \midrule
%  LLaVA1.5-7B~\citep{liu2023visual_llava} & 50.00         \basex{0.0}  & 15.40           \basex{0.0}  & 77.10 \basex{0.0}  & 100.6 \basex{0.0} \\
%   \textbf{+ AID (Ours)}                  & \textbf{41.80} \down{8.2}   & \textbf{13.00} \down{2.4}   & 77.10  \down{0.0}   & 96.80   \down{3.8} \\ 
% \midrule 
%  InstructBLIP~\citep{dai2023instructblip} & 57.2 \basex{0.0}         & \textbf{24.6} \basex{0.0}  & 66.3 \basex{0.0}  & 108.7 \basex{0.0} \\
%     \textbf{+ AID (Ours)}               & \textbf{52.8} \down{4.4} & \textbf{23.4} \down{1.2} & 65.3 \down{1.0} & 109.6 \up{0.9} \\
% \midrule
%  MiniGPT4~\citep{zhu2023minigpt4}      & 36.6 \basex{0.0}         & 12.8 \basex{0.0}         & 57.7 \basex{0.0} & 81 \basex{0.0} \\
%    \textbf{+ AID (Ours)}               & \textbf{32.2} \down{4.4} & \textbf{11.7} \down{1.1} & 56.8 \down{0.9} & 77.4 \down{3.6} \\
% \bottomrule
% \end{tabular}}
% % \vspace{-5pt}
% \caption{Results on CHAIRS of dataset. Best-performing method per model size and dataset is highlighted in bold; arrows indicate improvement or degradation over the baseline, where lower values indicate better performance.}
% \label{tab:res_chairs_5000}
% \end{table*}

\begin{table*}[h!]
\centering
\small
\resizebox{0.5 \linewidth}{!}{
\begin{tabular}{lllll}
\toprule
\multirow{2}{*}[-0.5ex]{\textbf{Method}} & \multicolumn{3}{c}{\quad\textbf{CHAIRs}}  \\
\cmidrule{2-4}				
 & \bf CHAIRs\down & \bf CHAIRi\down & \bf Length \\
\midrule
 LLaVA1.5-7B~\citep{liu2023visual_llava} & 50.80         \basex{0.0}  & 14.10           \basex{0.0}  & 100.50 \basex{0.0} \\
  \rowcolor{aliceblue} \textbf{+ AID (Ours)}                  & \textbf{46.10} \down{4.7}   & \textbf{12.90} \down{1.2}     & 97.00   \down{3.8} \\ 
\bottomrule
\end{tabular}}
% \vspace{-5pt}
\caption{Results on CHAIRS of MSCOCO val2017 dataset. Best-performing method per model size and dataset is highlighted in bold; arrows indicate improvement or degradation over the baseline, where lower values indicate better performance.}
\label{tab:res_chairs_5000}
\end{table*}

\noindent\textbf {The impact of instruction format.} To assess the extent of attention hijacking under varying instruction lengths and content, we conducted the following experiments.

\romannumeral1) 
As shown in Fig.~\ref{fig:instruction_len} (a), attention hijacking occurs across all instruction lengths (3-19), with a slight increase as length grows. We conclude that Attention hijacking is insensitive to instruction format or length, and AID is effective across diverse instructions.
This is due to the self-attention mechanism, where earlier parts of the instruction accumulate visual information for later parts

\romannumeral2) 
As demonstrated in Fig.~\ref{fig:instruction_len} (b) and (c), {various types of instructions($I1 - I5$) consistently trigger different degrees of attention hijacking, which AID effectively mitigates}. when given the instruction (I3)``Please provide a detailed description of elements in this image.", the CHAIRs and CHAIRi scores with AID are 42.8\%/13.5\%, compared to 50.2\%/15.1\% without AID. This variation is attributed to differences in Instruction-to-Visual Alignment Strength across instructions and images.

\begin{figure}[h]
% \vspace{-0.45cm}
    \setlength{\abovecaptionskip}{0.cm}  
    \setlength{\belowcaptionskip}{-0.2cm}
    \centering
    \includegraphics[width=1\linewidth]{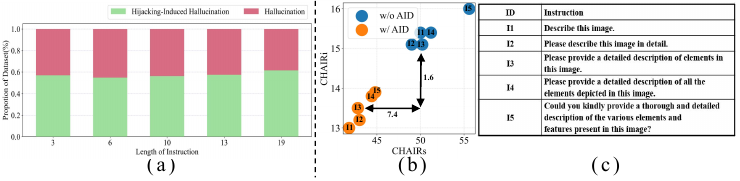}
    \caption{
    Attention hijacking under various formats of instruction.
    % Effect of Number of known classes \& Sample quality. K and U means average targeted attack success rate on known classes and unknown classes respectively.
    }
    \label{fig:instruction_len}
    % \vspace{-0.3cm}
\end{figure}

\subsection{Reproducibility}
\paragraph{Implementation details.} We employed beam search as the default decoding strategy across all benchmark evaluations. For the hallucination benchmarks (POPE and CHAIR) and general-purpose benchmarks (MME, VizWiz-VQA, MMBench, MM-Vet, and LLaVA-Bench (in-the-wild)), questions from the annotation files were used as prompts, formatted to fit the chat templates of each respective LVLM.

\begin{table*}[h!]
\centering
\small
\resizebox{1.0 \linewidth}{!}{
\begin{tabular}{llllllll}
\toprule
\multirow{2}{*}[-0.5ex]{\textbf{Method}} & \multicolumn{6}{c}{\quad\quad\quad\quad\textbf{MMBench-Dev-EN}}  \\
\cmidrule(lr){2-8}					
 & \bf AR & \bf CP & \bf FP-C & \bf FP-S  &\bf LR  &\bf RR  &\bf Overall \\
\midrule
 LLaVA1.5-7B & 72.86 \basex{0.0}  & 75.68 \basex{0.0}  & 58.04 \basex{0.0}  & 63.48 \basex{0.0} & 28.81 \basex{0.0}  & 51.30 \basex{0.0}  & 62.80 \basex{0.0} \\
  + VCD~\citep{leng2023mitigating_vcd} & 60.30 & 68.58 & 51.75 & 53.24 & 18.64 & 48.70 & 54.21 \\
  + OPERA~\citep{huang2023opera}  & 69.85 & 75.00 & 56.64 & 66.21 & 28.81 & 53.04 & 62.80 \\
  \rowcolor{aliceblue} \textbf{+ AID (Ours)} & 73.36 \up{0.5} & 75.67 \basex{0.0} & 57.34 \downbad{0.7} & 67.57 \up{4.1} & 31.35 \up{2.5} & 53.04 \up{1.7} & \textbf{64.26} \up{1.4} \\ 
\midrule
 GLM-4V-9B & 88.44 \basex{0.0}  & 86.49 \basex{0.0}  & 69.93 \basex{0.0} & 85.67 \basex{0.0} & 66.10 \basex{0.0}  & 85.22 \basex{0.0}  & 82.39 \basex{0.0}  \\
  + VCD~\citep{leng2023mitigating_vcd} & 86.43 & 85.47 & 68.53 & 84.64 & 61.86 & 81.74 & 80.58 \\
  + OPERA~\citep{huang2023opera}  & - & - & - & - & - & - & - \\
   \rowcolor{aliceblue} \textbf{+ AID (Ours)}  & 88.94 \up{0.5} & 86.49 \basex{0.0} & 70.63 \up{0.7} & 86.01 \up{0.4} & 66.10 \basex{0.0} & 85.22 \basex{0.0} & \textbf{82.65} \up{0.3} \\
% \midrule 
%  Qwen-VL-10B & 60.30 \basex{0.0}  & 71.28 \basex{0.0}  & 45.45 \basex{0.0}  & 62.80 \basex{0.0}  & 28.81 \basex{0.0}  & 38.26 \basex{0.0} & \textbf{56.53} \basex{0.0} \\
%    + VCD~\citep{leng2023mitigating_vcd} & 34.67 & 52.36 & 20.28 & 55.63 & 11.86 & 22.61 & 39.18 \\
%    + OPERA~\citep{huang2023opera}  & - & - & - & - & - & - & - \\
%     \textbf{+ AID (Ours)}  & 61.51 \up{1.2} & 71.28 \basex{0.0} & 44.06 \downbad{1.4} & 62.80 \basex{0.0} & 27.77 \downbad{1.0} & 38.26 \basex{0.0} & 56.44 \downbad{0.1} \\
\bottomrule
\end{tabular}}
\vspace{-5pt}
\caption{Results on MMBench dataset. Best-performing method per model size and dataset is highlighted in bold; arrows indicate improvement or degradation over the baseline, where lower values indicate better performance.}
\label{tab:res_mmbench22}
\end{table*}

Specifically, we utilized the COCO, A-OKVQA, and GQA datasets for POPE evaluation, and MMBench\_DEV\_EN for MMBench. In the MM-Vet evaluation, we used an online evaluator powered by OpenAI GPT-4 to assess generated results, while for LLaVA-Bench (in-the-wild), we employed OpenAI’s model gpt4-1106-preview via API. For CHAIR, a randomly sampled image set from the COCO Val2014 dataset was used across all three models, with the prompt "Please describe this image in detail." We sampled three different sets of images using different random seeds and evaluated performance by calculating the mean and standard deviation of the results. 
Due to OPERA's reliance on older versions of Torch and Transformers, it was incompatible with Qwen and GLM models, and thus experiments involving these models were not conducted. Additionally, our method introduces two hyperparameters: the informative layer l for activation calculations and the factor $\lambda$ to control the influence of entropy on the next token probability distribution. To map the hidden states from selected layers l to vocabulary tokens, we chose intermediate layers based on the model's depth (e.g., layers 5 to 16 for vicuna-7b, which has 32 layers), and we set $\lambda$ as a fixed value (e.g., 0.75). All parameter settings adhered to the default configurations specified in the respective papers and code repositories.

\begin{table*}[h!]
\centering
\small
\resizebox{0.7 \linewidth}{!}{
\begin{tabular}{llllll}
\toprule
\multirow{2}{*}[-0.5ex]{\textbf{Method}} & \multicolumn{4}{c}{\quad\quad\quad\quad\textbf{LLaVABench (in-the-wild)}}  \\
\cmidrule(lr){2-5}					
 & \bf Average & \bf All\_1 & \bf All\_2 & \bf All\_3 \\
\midrule
 LLaVA1.5-7B & 64.80 \basex{0.0}  & 63.40 \basex{0.0}  & 80.20 \basex{0.0}  & 50.80 \basex{0.0} \\
  + VCD~\citep{leng2023mitigating_vcd} & 63.20 \downbad{1.6} & 59.10 \downbad{4.3} & 82.00 \up{1.8} & 48.50 \downbad{2.3} \\
  + OPERA~\citep{huang2023opera}  & 64.30 \downbad{0.5} & 59.80 \downbad{3.6} & 83.30 \up{3.1} & 49.80 \downbad{1.0} \\
  \rowcolor{aliceblue} \textbf{+ AID (Ours)} & \textbf{65.30} \up{0.5} & 64.10 \up{0.7} & 80.20 \basex{0.0} & 51.50 \up{0.7} \\ 
\midrule
 Qwen-VL-Chat & 68.50 \basex{0.0}  & 70.40 \basex{0.0}  & 79.30 \basex{0.0} & 55.80 \basex{0.0} \\
  + VCD~\citep{leng2023mitigating_vcd} & 53.77 \downbad{14.7} & 41.00 \downbad{29.4} & 85.30 \up{6.0} & 35.00 \downbad{20.8} \\
  + OPERA~\citep{huang2023opera}  & - & - & - & - \\
   \rowcolor{aliceblue} \textbf{+ AID (Ours)}  & \textbf{69.50} \up{1.0} & 69.50 \downbad{0.9} & 82.00 \up{2.7} & 57.00 \up{1.2} \\
\midrule 
 GLM-4V-9B & 75.30 \basex{0.0}  & 88.40 \basex{0.0}  & 73.00 \basex{0.0}  & 64.50 \basex{0.0} \\
   + VCD~\citep{leng2023mitigating_vcd} & 74.23 \downbad{1.1} & 86.70 \downbad{1.7} & 72.80 \downbad{0.2} & 63.20 \downbad{1.3} \\
   + OPERA~\citep{huang2023opera}  & - & - & - & - \\
    \rowcolor{aliceblue} \textbf{+ AID (Ours)}  & \textbf{76.9} \up{1.6} & 88.90 \up{0.5} & 75.20 \up{2.2} & 66.60 \up{2.1} \\
\bottomrule
\end{tabular}}
\vspace{-5pt}
\caption{Results on LLaVABench (in-the-wild) dataset. Best-performing method per model size and dataset is highlighted in bold; arrows indicate improvement or degradation over the baseline.}
\label{tab:res_llavabench}
\end{table*}

\section{Experiments and Computational Resources.}

\subsection{Experimental Code.}
To promote transparency and ensure the reproducibility of our work, we will release all experimental code, datasets, and detailed tutorials necessary for replicating our experiments. Our goal is to make it straightforward for researchers and practitioners to reproduce our results, regardless of their technical background. Additionally, by providing comprehensive documentation and clear guidelines, we aim to facilitate the extension of our method to other models and architectures, enabling the broader research community to explore its potential applications and improvements. We believe that open and reproducible research is essential for advancing the field and fostering collaboration.

\subsection{Computational Resources.}
 The decoding process of LVLMs and all experiments are performed on 8 V100 GPUs.

\section{Case Study}
\label{apx:visualization}
This case study aims to evaluate and present various benchmark cases across multiple domains
systematically.

\subsection{Detail Description Study}
Additional case studies are presented to illustrate the effectiveness of our AID of generative task on MSCOCO dataset, as shown in Fig~\ref{fig:long_case1}, Fig~\ref{fig:long_case2}, Fig~\ref{fig:long_case3}, Fig~\ref{fig:long_case4}, Fig~\ref{fig:long_case5}, and Fig~\ref{fig:short_case1}.

\begin{figure*}[h]
    \centering
    \includegraphics[width=1\linewidth]{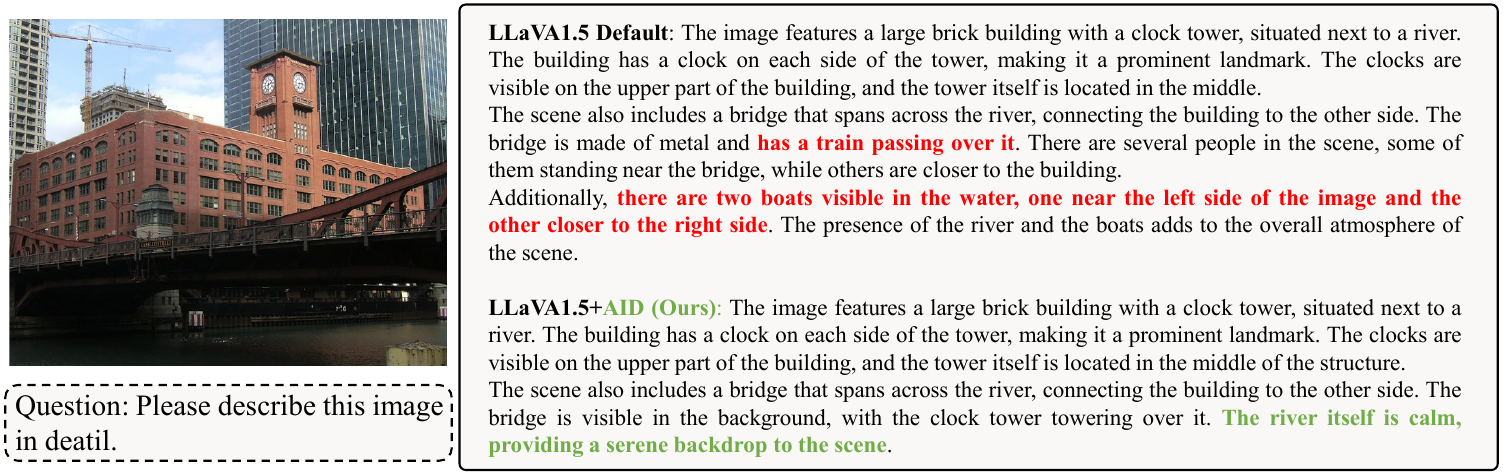}
    \caption{A case study comparing the levels of hallucination among various baselines.}
    \label{fig:long_case1}
\end{figure*}

\begin{figure*}[h]
    \centering
    \includegraphics[width=1\linewidth]{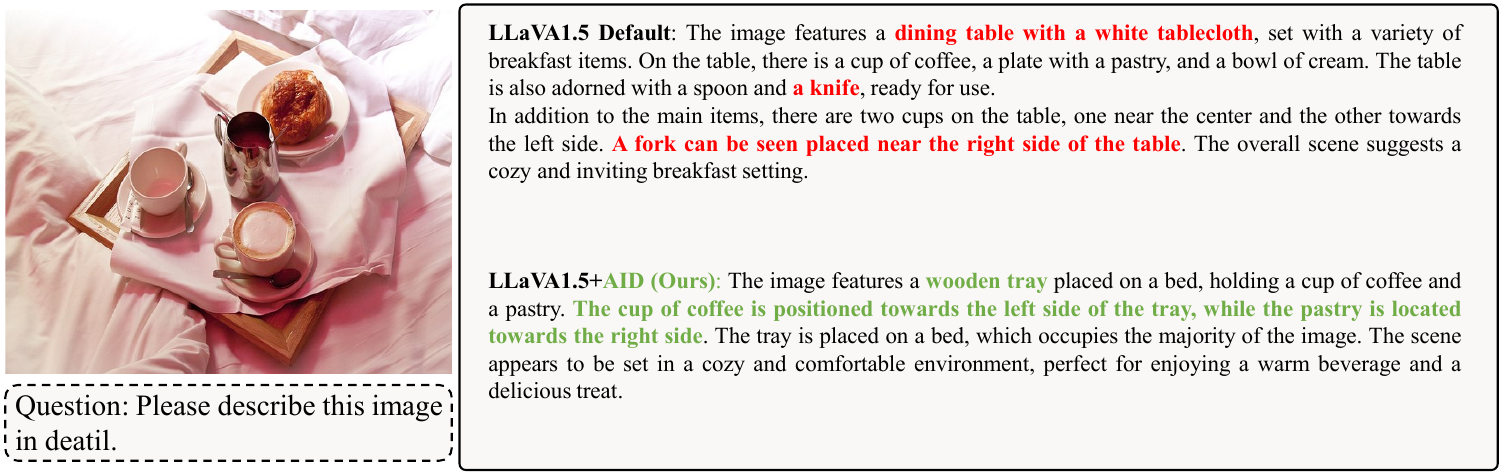}
    \caption{A case study comparing the levels of hallucination among various baselines.}
    \label{fig:long_case2}
\end{figure*}

\begin{figure*}[h]
    \centering
    \includegraphics[width=1\linewidth]{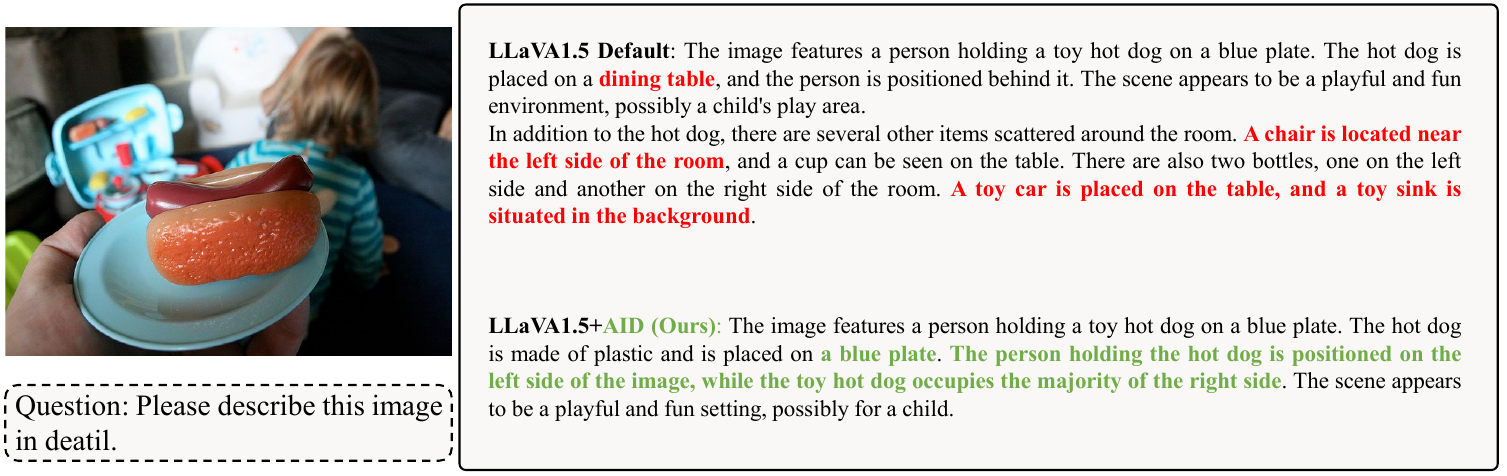}
    \caption{A case study comparing the levels of hallucination among various baselines.}
    \label{fig:long_case3}
\end{figure*}

\begin{figure*}[h]
    \centering
    \includegraphics[width=1\linewidth]{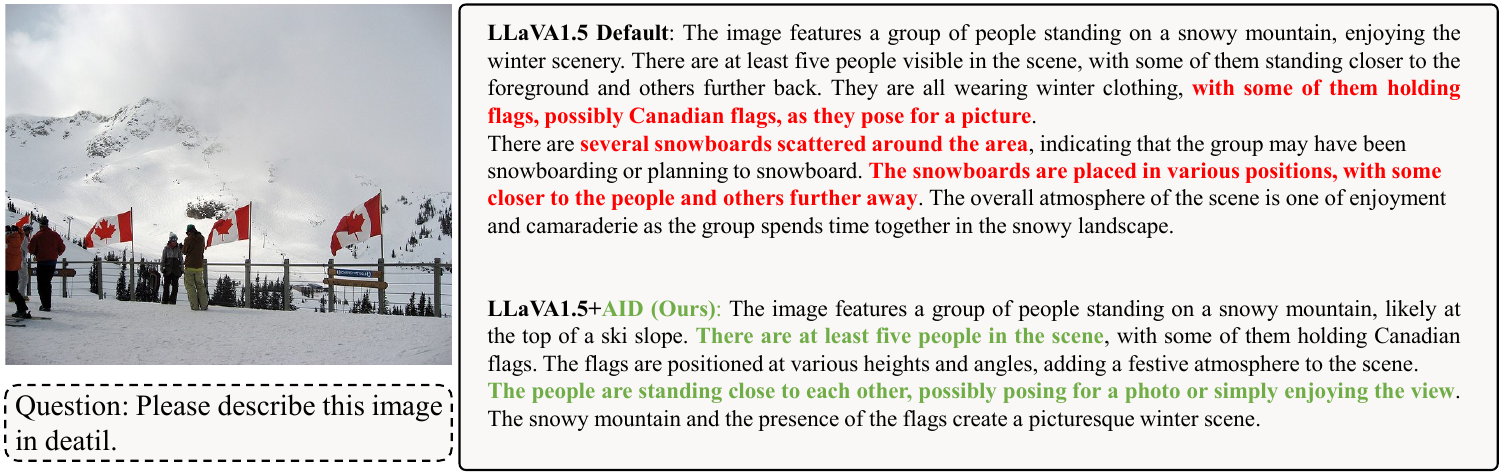}
    \caption{A case study comparing the levels of hallucination among various baselines.}
    \label{fig:long_case4}
\end{figure*}

\begin{figure*}[h]
    \centering
    \includegraphics[width=1\linewidth]{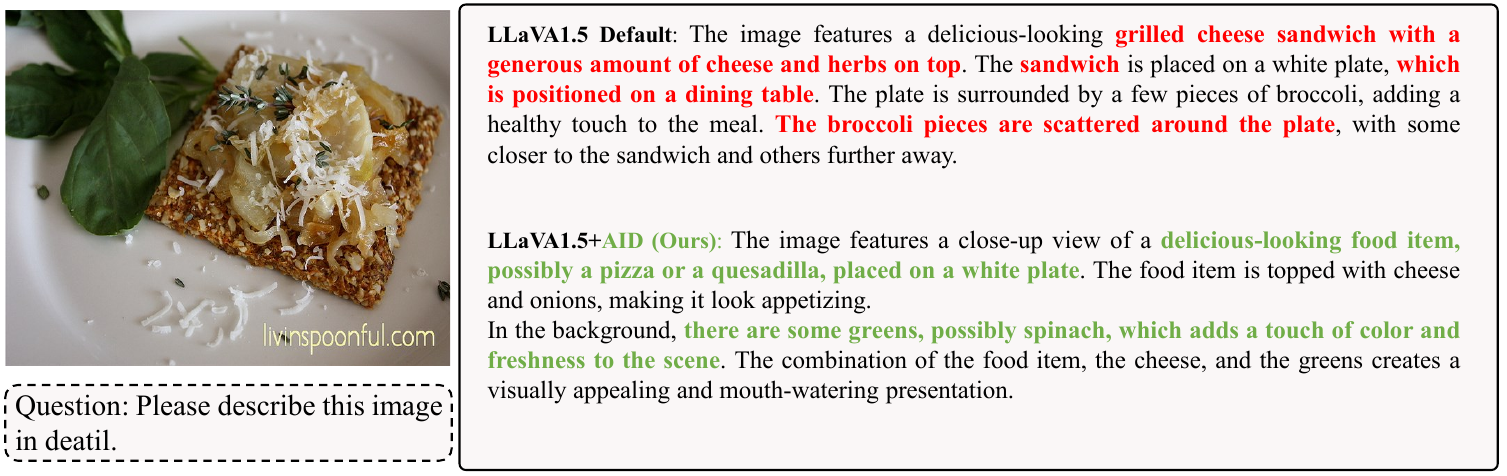}
    \caption{A case study comparing the levels of hallucination among various baselines.}
    \label{fig:long_case5}
\end{figure*}

\begin{figure*}[h]
    \centering
    \includegraphics[width=1\linewidth]{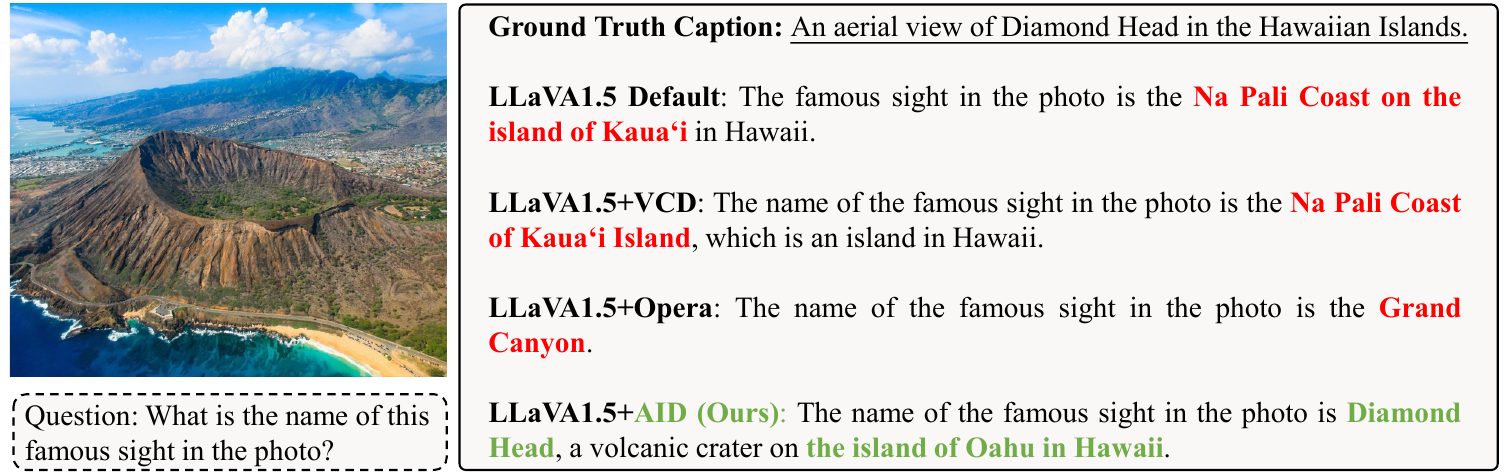}
    \caption{A case study comparing the levels of hallucination among various baselines.}
    \label{fig:short_case1}
\end{figure*}

\subsection{Discriminate Problem Study}
Furthermore, we provide extra case studies to illustrate the effectiveness of our AID in discriminate task on the POPE benchmark, as shown in Fig.~\ref{fig:pope_case1},Fig.~\ref{fig:pope_case2}, and Fig.~\ref{fig:pope_case3}.

\begin{figure*}[h]
    \centering
    \includegraphics[width=0.95\linewidth]{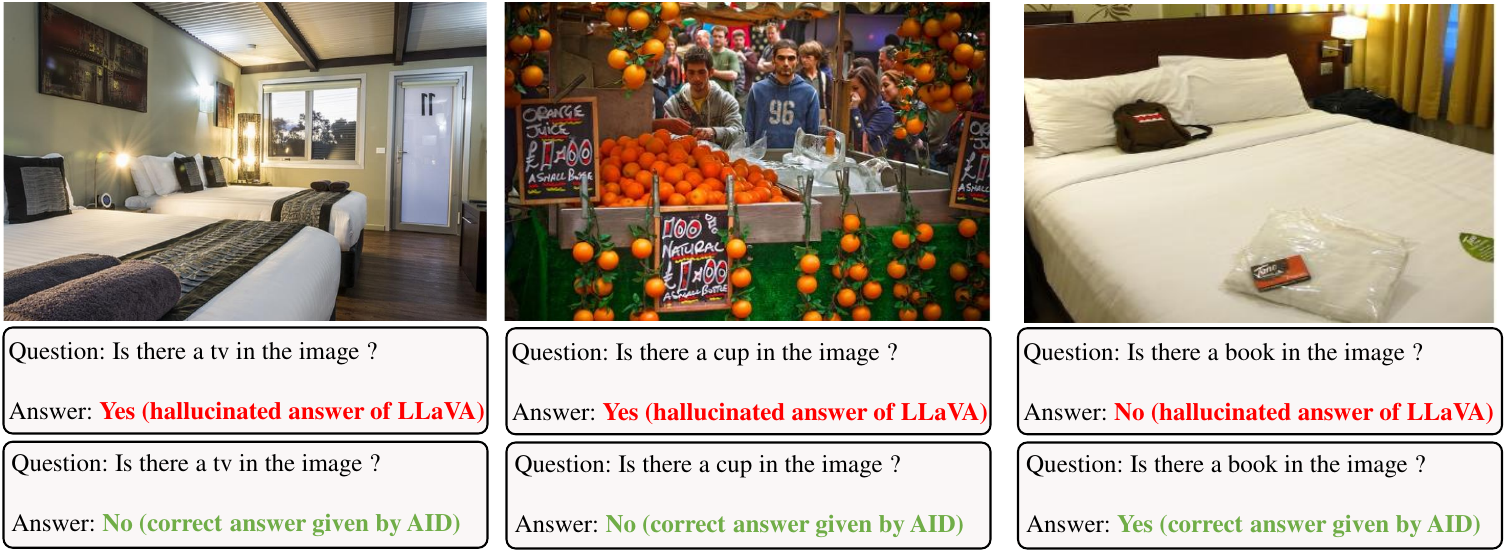}
    \caption{A case study comparing the levels of hallucination among various baselines.}
    \label{fig:pope_case1}
\end{figure*}

\begin{figure*}[h]
    \centering
    \includegraphics[width=0.95\linewidth]{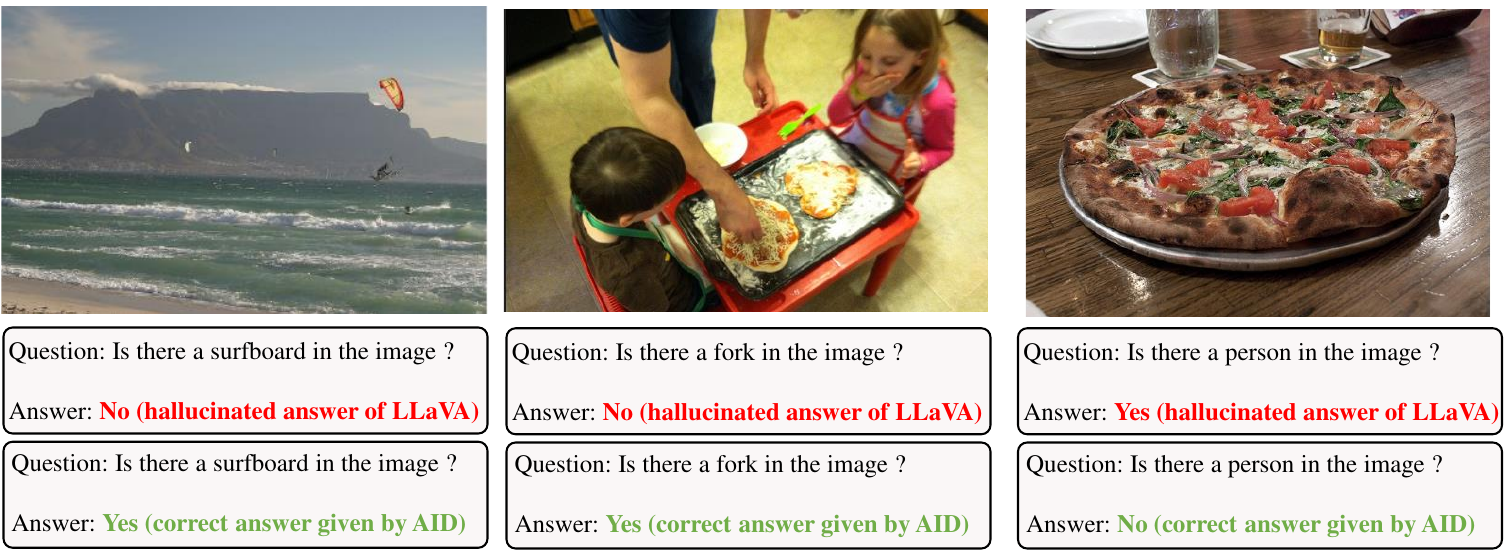}
    \caption{A case study comparing the levels of hallucination among various baselines.}
    \label{fig:pope_case2}
\end{figure*}

\begin{figure*}[h]
    \centering
    \includegraphics[width=0.95\linewidth]{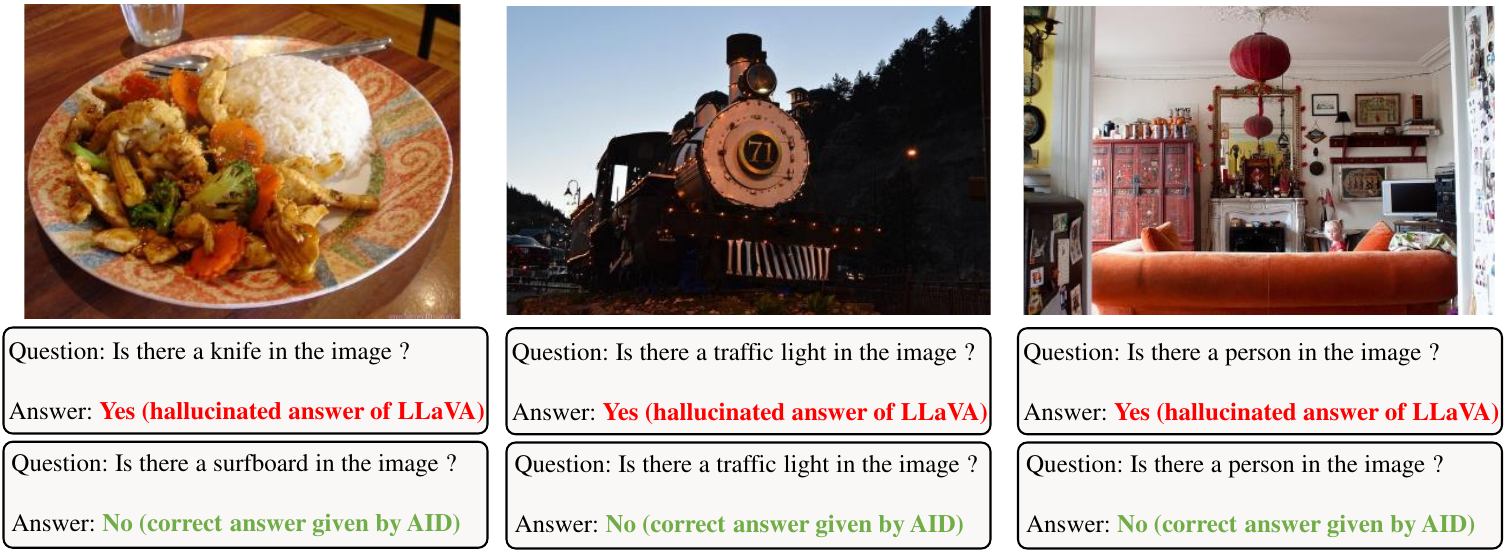}
    \caption{A case study comparing the levels of hallucination among various baselines.}
    \label{fig:pope_case3}
\end{figure*}

\begin{figure*}[h]
    \centering
    \includegraphics[width=0.8\linewidth]{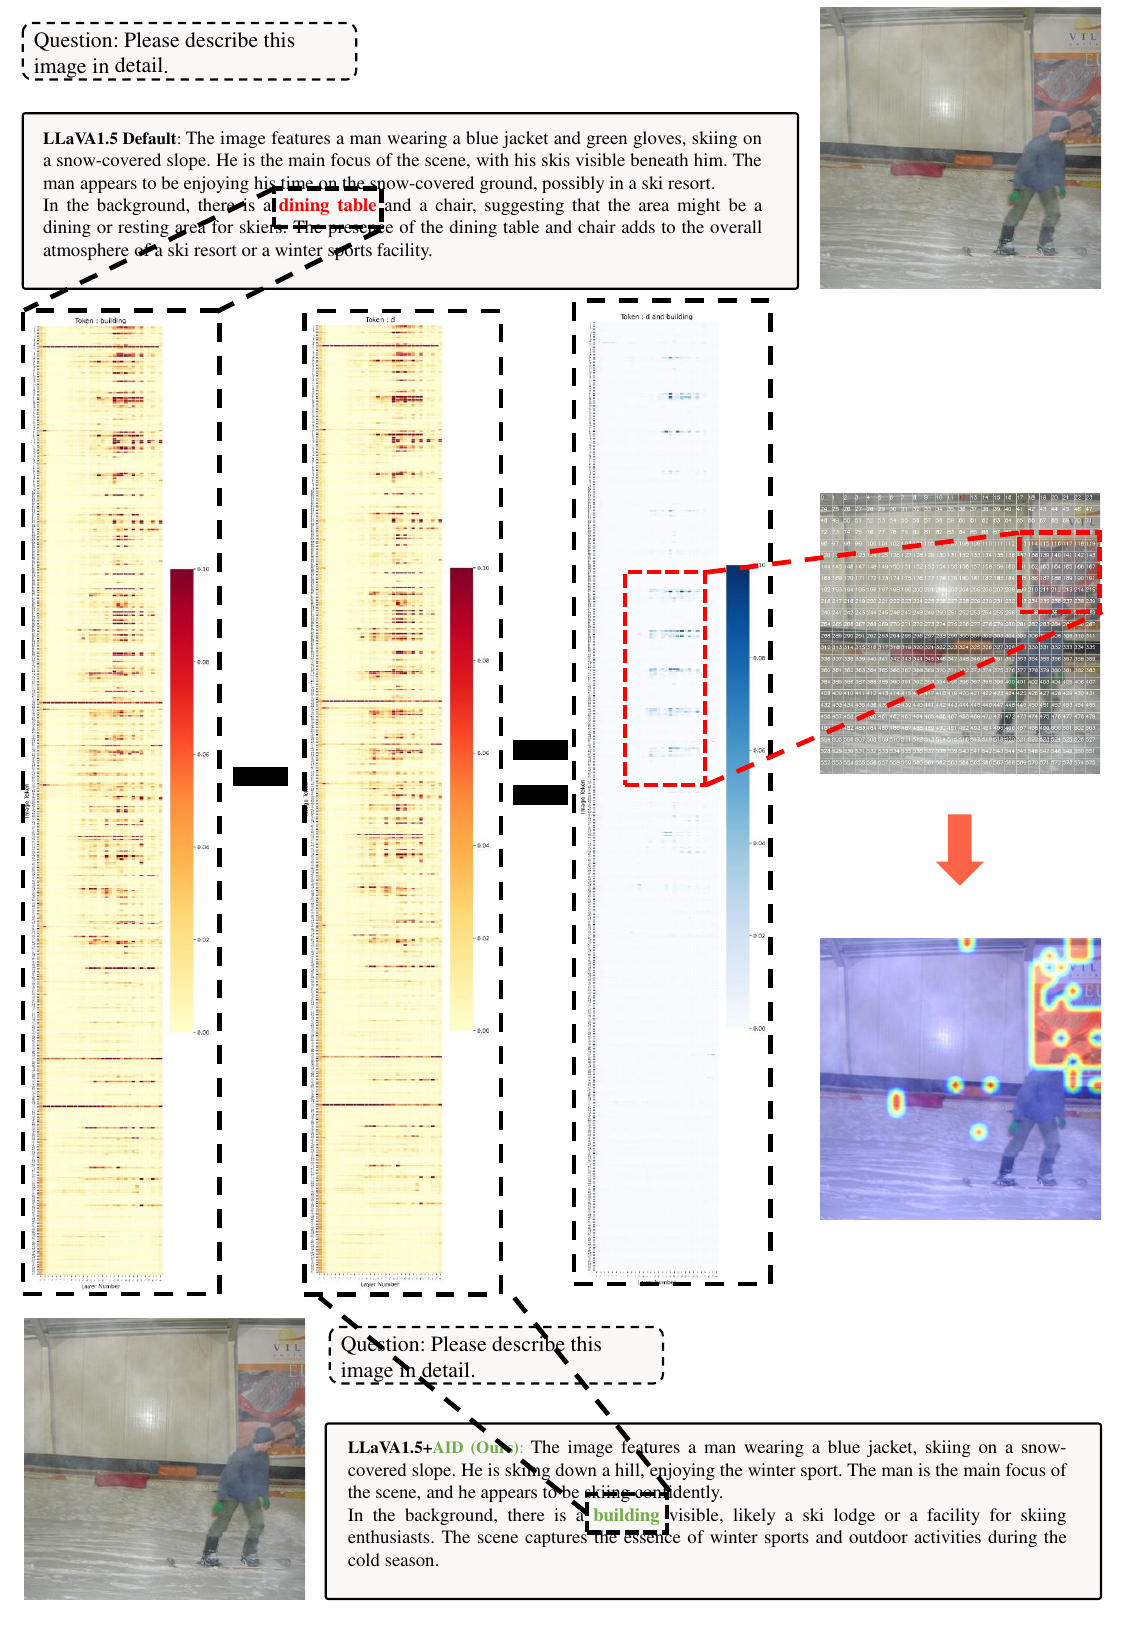}
    \caption{A case study comparing the changes in the Attention Map.}
    \label{fig:change_attention_map}
\end{figure*}

\section{Attention Map Study}
\label{apx:attention_map}
% To validate the effectiveness of our AID in isolating the influence of identified hijackers, thereby allowing the model to independently explore appropriate visual interaction patterns, we visualize the changing of visual attention map before and after utilizing our AID in Fig.~\ref{fig:change_attention_map}.

To validate the effectiveness of our AID mechanism in isolating the influence of identified hijackers and enabling the model to independently explore appropriate visual interaction patterns, we visualized the changes in visual attention maps of the output tokens before and after applying AID. Specifically, we visualized the visual attention maps of the token corresponding to dining table across all layers, as shown in Fig.~\ref{fig:change_attention_map}.

\subsection{Changes in the Attention Map}
Observed in Fig.~\ref{fig:change_attention_map}, the default LLaVA model generates a hallucinatory object, dining table, when describing the given image. After applying our AID, the model outputs the correct object, building, which directly replaces the hallucinated dining table. We then visualized the attention maps for the building token. By subtracting the two attention maps, we obtained a visual attention difference map, displayed in the middle. This attention difference map clearly corresponds to a localized interfering region in the original image. This visualization demonstrates that AID effectively redistributes the localized erroneous attention originally hijacked, enabling the model to infer the correct object based on the appropriate context.

% As illustrated in Fig.~\ref{fig:change_attention_map}, our proposed AID enables the model to move beyond reliance on local visual regions, allowing it to effectively capture and leverage contextual information within the image.

\end{appendices}
