# Supplementary material for: Attention Hijackers: Detect and Disentangle Attention Hijacking in LVLMs for Hallucination Mitigation
Source: arXiv:2503.08216 source file (2025-03-14)
Supplement: Supplementary file 2 [file Appendix_CHIAIRS.tex]

\begin{table*}[h!]
\centering
\small
\resizebox{0.5 \linewidth}{!}{
\begin{tabular}{llll}
\toprule
\multirow{2}{*}[-0.5ex]{\textbf{Method}} & \multicolumn{3}{c}{\quad\textbf{CHAIRs}}  \\
\cmidrule{2-4}				
 & \bf CHAIRs\down & \bf CHAIRi\down   & \bf Length \\
\midrule
 LLaVA1.5-7B                            & 50.00         \basex{0.0}  & 15.40           \basex{0.0}    & 100.6 \basex{0.0} \\
  + VCD~\citep{leng2023mitigating_vcd}  & 48.60         \down{1.4}   & 14.90           \down{0.5}     & 100.4 \down{0.2} \\
  + OPERA~\citep{huang2023opera}        & 47.80         \down{2.2}   & 14.60           \down{0.8}     & 98.60  \down{2.0} \\
  \rowcolor{aliceblue} \textbf{+ AID (Ours)}                 & \textbf{41.80} \down{8.2}   & \textbf{13.00} \down{2.4}     & 96.80   \down{3.8} \\ 
\midrule 
 GLM-4V-9B                              & 40.40 \basex{0.0}         & \textbf{9.00} \basex{0.0}    & 218.20 \basex{0.0} \\
   + VCD~\citep{leng2023mitigating_vcd} & 42.20 \upbad{1.8}         & 9.60 \upbad{0.6} &  239.80 \upbad{21.6} \\
   + OPERA~\citep{huang2023opera}       & - & -  & - \\
    \rowcolor{aliceblue} \textbf{+ AID (Ours)}               & \textbf{38.20} \down{2.2} & \textbf{8.80} \down{0.2} & 210.00 \down{6.2} \\
\midrule
 Qwen-VL-10B                           & 10.20 \basex{0.0}         & 7.20 \basex{0.0}          & 22.50 \basex{0.0} \\
  + VCD~\citep{leng2023mitigating_vcd} & 13.00 \upbad{2.8}        & 12.3 \upbad{5.1}          & 115.7 \upbad{93.2} \\
  + OPERA~\citep{huang2023opera}       & - & -  & - \\
   \rowcolor{aliceblue} \textbf{+ AID (Ours)}               & \textbf{5.200} \down{5.0} & \textbf{3.30} \down{3.9}  & 12.90 \down{9.6} \\
\bottomrule
\end{tabular}}
% \vspace{-5pt}
\caption{Results on CHAIRS dataset. Best-performing method per model size and dataset is highlighted in bold; arrows indicate improvement or degradation over the baseline, where lower values indicate better performance.}
\label{tab:res_chairs}
\end{table*}
