# Supplementary material for: Attention Hijackers: Detect and Disentangle Attention Hijacking in LVLMs for Hallucination Mitigation
Source: arXiv:2503.08216 source file (2025-03-14)
Supplement: Supplementary file 3 [file Appendix_CHIAIRS_5000.tex]

\begin{table*}[h!]
\centering
\small
\resizebox{0.5 \linewidth}{!}{
\begin{tabular}{lllll}
\toprule
\multirow{2}{*}[-0.5ex]{\textbf{Method}} & \multicolumn{3}{c}{\quad\textbf{CHAIRs}}  \\
\cmidrule{2-4}				
 & \bf CHAIRs\down & \bf CHAIRi\down & \bf Length \\
\midrule
 LLaVA1.5-7B~\citep{liu2023visual_llava} & 50.80         \basex{0.0}  & 14.10           \basex{0.0}  & 100.50 \basex{0.0} \\
  \rowcolor{aliceblue} \textbf{+ AID (Ours)}                  & \textbf{46.10} \down{4.7}   & \textbf{12.90} \down{1.2}     & 97.00   \down{3.8} \\ 
\bottomrule
\end{tabular}}
% \vspace{-5pt}
\caption{Results on CHAIRS of MSCOCO val2017 dataset. Best-performing method per model size and dataset is highlighted in bold; arrows indicate improvement or degradation over the baseline, where lower values indicate better performance.}
\label{tab:res_chairs_5000}
\end{table*}
