# Supplementary material for: Attention Hijackers: Detect and Disentangle Attention Hijacking in LVLMs for Hallucination Mitigation
Source: arXiv:2503.08216 source file (2025-03-14)
Supplement: Supplementary file 4 [file Appendix_CHIAIRS_models.tex]

\begin{table*}[h!]
\centering
\small
\resizebox{0.5 \linewidth}{!}{
\begin{tabular}{lllll}
\toprule
\multirow{2}{*}[-0.5ex]{\textbf{Method}} & \multicolumn{3}{c}{\quad\textbf{CHAIRs}}  \\
\cmidrule{2-4}				
 & \bf CHAIRs\down & \bf CHAIRi\down  & \bf Length \\
\midrule
 LLaVA1.5-7B~\citep{liu2023visual_llava} & 50.00         \basex{0.0}  & 15.40           \basex{0.0}    & 100.6 \basex{0.0} \\
  \rowcolor{aliceblue} \textbf{+ AID (Ours)}                  & \textbf{41.80} \down{8.2}   & \textbf{13.00} \down{2.4}    & 96.80   \down{3.8} \\ 
\midrule 
 InstructBLIP~\citep{dai2023instructblip} & 57.2 \basex{0.0}         & \textbf{24.6} \basex{0.0}   & 108.7 \basex{0.0} \\
    \rowcolor{aliceblue} \textbf{+ AID (Ours)}               & \textbf{52.8} \down{4.4} & \textbf{23.4} \down{1.2}  & 109.6 \up{0.9} \\
\midrule
 MiniGPT4~\citep{zhu2023minigpt4}      & 36.6 \basex{0.0}         & 12.8 \basex{0.0}         & 81 \basex{0.0} \\
   \rowcolor{aliceblue} \textbf{+ AID (Ours)}               & \textbf{32.2} \down{4.4} & \textbf{11.7} \down{1.1}  & 77.4 \down{3.6} \\
\bottomrule
\end{tabular}}
% \vspace{-5pt}
\caption{Results on CHAIRS of dataset. Best-performing method per model size and dataset is highlighted in bold; arrows indicate improvement or degradation over the baseline, where lower values indicate better performance.}
\label{tab:res_chairs_5000}
\end{table*}

% \begin{table*}[h!]
% \centering
% \small
% \resizebox{0.7 \linewidth}{!}{
% \begin{tabular}{llllll}
% \toprule
% \multirow{2}{*}[-0.5ex]{\textbf{Method}} & \multicolumn{4}{c}{\quad\quad\textbf{CHAIRs}}  \\
% \cmidrule{2-5}				
%  & \bf CHAIRs & \bf CHAIRi & \bf Recall & \bf Len \\
% \midrule
%  LLaVA1.5-7B~\citep{liu2023visual_llava} & 50.00         \basex{0.0}  & 15.40           \basex{0.0}  & 77.10 \basex{0.0}  & 100.6 \basex{0.0} \\
%   \textbf{+ AID (Ours)}                  & \textbf{41.80} \down{8.2}   & \textbf{13.00} \down{2.4}   & 77.10  \down{0.0}   & 96.80   \down{3.8} \\ 
% \midrule 
%  InstructBLIP~\citep{dai2023instructblip} & 57.2 \basex{0.0}         & \textbf{24.6} \basex{0.0}  & 66.3 \basex{0.0}  & 108.7 \basex{0.0} \\
%     \textbf{+ AID (Ours)}               & \textbf{52.8} \down{4.4} & \textbf{23.4} \down{1.2} & 65.3 \down{1.0} & 109.6 \up{0.9} \\
% \midrule
%  MiniGPT4~\citep{zhu2023minigpt4}      & 36.6 \basex{0.0}         & 12.8 \basex{0.0}         & 57.7 \basex{0.0} & 81 \basex{0.0} \\
%    \textbf{+ AID (Ours)}               & \textbf{32.2} \down{4.4} & \textbf{11.7} \down{1.1} & 56.8 \down{0.9} & 77.4 \down{3.6} \\
% \bottomrule
% \end{tabular}}
% % \vspace{-5pt}
% \caption{Results on CHAIRS of dataset. Best-performing method per model size and dataset is highlighted in bold; arrows indicate improvement or degradation over the baseline, where lower values indicate better performance.}
% \label{tab:res_chairs_5000}
% \end{table*}
