# Supplementary material for: Attention Hijackers: Detect and Disentangle Attention Hijacking in LVLMs for Hallucination Mitigation
Source: arXiv:2503.08216 source file (2025-03-14)
Supplement: Supplementary file 5 [file Appendix_LLaVABench.tex]

\begin{table*}[h!]
\centering
\small
\resizebox{0.7 \linewidth}{!}{
\begin{tabular}{llllll}
\toprule
\multirow{2}{*}[-0.5ex]{\textbf{Method}} & \multicolumn{4}{c}{\quad\quad\quad\quad\textbf{LLaVABench (in-the-wild)}}  \\
\cmidrule(lr){2-5}					
 & \bf Average & \bf All\_1 & \bf All\_2 & \bf All\_3 \\
\midrule
 LLaVA1.5-7B & 64.80 \basex{0.0}  & 63.40 \basex{0.0}  & 80.20 \basex{0.0}  & 50.80 \basex{0.0} \\
  + VCD~\citep{leng2023mitigating_vcd} & 63.20 \downbad{1.6} & 59.10 \downbad{4.3} & 82.00 \up{1.8} & 48.50 \downbad{2.3} \\
  + OPERA~\citep{huang2023opera}  & 64.30 \downbad{0.5} & 59.80 \downbad{3.6} & 83.30 \up{3.1} & 49.80 \downbad{1.0} \\
  \rowcolor{aliceblue} \textbf{+ AID (Ours)} & \textbf{65.30} \up{0.5} & 64.10 \up{0.7} & 80.20 \basex{0.0} & 51.50 \up{0.7} \\ 
\midrule
 Qwen-VL-Chat & 68.50 \basex{0.0}  & 70.40 \basex{0.0}  & 79.30 \basex{0.0} & 55.80 \basex{0.0} \\
  + VCD~\citep{leng2023mitigating_vcd} & 53.77 \downbad{14.7} & 41.00 \downbad{29.4} & 85.30 \up{6.0} & 35.00 \downbad{20.8} \\
  + OPERA~\citep{huang2023opera}  & - & - & - & - \\
   \rowcolor{aliceblue} \textbf{+ AID (Ours)}  & \textbf{69.50} \up{1.0} & 69.50 \downbad{0.9} & 82.00 \up{2.7} & 57.00 \up{1.2} \\
\midrule 
 GLM-4V-9B & 75.30 \basex{0.0}  & 88.40 \basex{0.0}  & 73.00 \basex{0.0}  & 64.50 \basex{0.0} \\
   + VCD~\citep{leng2023mitigating_vcd} & 74.23 \downbad{1.1} & 86.70 \downbad{1.7} & 72.80 \downbad{0.2} & 63.20 \downbad{1.3} \\
   + OPERA~\citep{huang2023opera}  & - & - & - & - \\
    \rowcolor{aliceblue} \textbf{+ AID (Ours)}  & \textbf{76.9} \up{1.6} & 88.90 \up{0.5} & 75.20 \up{2.2} & 66.60 \up{2.1} \\
\bottomrule
\end{tabular}}
\vspace{-5pt}
\caption{Results on LLaVABench (in-the-wild) dataset. Best-performing method per model size and dataset is highlighted in bold; arrows indicate improvement or degradation over the baseline.}
\label{tab:res_llavabench}
\end{table*}
