# Supplementary material for: Attention Hijackers: Detect and Disentangle Attention Hijacking in LVLMs for Hallucination Mitigation
Source: arXiv:2503.08216 source file (2025-03-14)
Supplement: Supplementary file 6 [file Appendix_MMBench.tex]

\begin{table*}[h!]
\centering
\small
\resizebox{1.0 \linewidth}{!}{
\begin{tabular}{llllllll}
\toprule
\multirow{2}{*}[-0.5ex]{\textbf{Method}} & \multicolumn{6}{c}{\quad\quad\quad\quad\textbf{MMBench-Dev-EN}}  \\
\cmidrule(lr){2-8}					
 & \bf AR & \bf CP & \bf FP-C & \bf FP-S  &\bf LR  &\bf RR  &\bf Overall \\
\midrule
 LLaVA1.5-7B & 72.86 \basex{0.0}  & 75.68 \basex{0.0}  & 58.04 \basex{0.0}  & 63.48 \basex{0.0} & 28.81 \basex{0.0}  & 51.30 \basex{0.0}  & 62.80 \basex{0.0} \\
  + VCD~\citep{leng2023mitigating_vcd} & 60.30 & 68.58 & 51.75 & 53.24 & 18.64 & 48.70 & 54.21 \\
  + OPERA~\citep{huang2023opera}  & 69.85 & 75.00 & 56.64 & 66.21 & 28.81 & 53.04 & 62.80 \\
  \rowcolor{aliceblue} \textbf{+ AID (Ours)} & 73.36 \up{0.5} & 75.67 \basex{0.0} & 57.34 \downbad{0.7} & 67.57 \up{4.1} & 31.35 \up{2.5} & 53.04 \up{1.7} & \textbf{64.26} \up{1.4} \\ 
\midrule
 GLM-4V-9B & 88.44 \basex{0.0}  & 86.49 \basex{0.0}  & 69.93 \basex{0.0} & 85.67 \basex{0.0} & 66.10 \basex{0.0}  & 85.22 \basex{0.0}  & 82.39 \basex{0.0}  \\
  + VCD~\citep{leng2023mitigating_vcd} & 86.43 & 85.47 & 68.53 & 84.64 & 61.86 & 81.74 & 80.58 \\
  + OPERA~\citep{huang2023opera}  & - & - & - & - & - & - & - \\
   \rowcolor{aliceblue} \textbf{+ AID (Ours)}  & 88.94 \up{0.5} & 86.49 \basex{0.0} & 70.63 \up{0.7} & 86.01 \up{0.4} & 66.10 \basex{0.0} & 85.22 \basex{0.0} & \textbf{82.65} \up{0.3} \\
% \midrule 
%  Qwen-VL-10B & 60.30 \basex{0.0}  & 71.28 \basex{0.0}  & 45.45 \basex{0.0}  & 62.80 \basex{0.0}  & 28.81 \basex{0.0}  & 38.26 \basex{0.0} & \textbf{56.53} \basex{0.0} \\
%    + VCD~\citep{leng2023mitigating_vcd} & 34.67 & 52.36 & 20.28 & 55.63 & 11.86 & 22.61 & 39.18 \\
%    + OPERA~\citep{huang2023opera}  & - & - & - & - & - & - & - \\
%     \textbf{+ AID (Ours)}  & 61.51 \up{1.2} & 71.28 \basex{0.0} & 44.06 \downbad{1.4} & 62.80 \basex{0.0} & 27.77 \downbad{1.0} & 38.26 \basex{0.0} & 56.44 \downbad{0.1} \\
\bottomrule
\end{tabular}}
\vspace{-5pt}
\caption{Results on MMBench dataset. Best-performing method per model size and dataset is highlighted in bold; arrows indicate improvement or degradation over the baseline, where lower values indicate better performance.}
\label{tab:res_mmbench22}
\end{table*}
