# Supplementary material for: Attention Hijackers: Detect and Disentangle Attention Hijacking in LVLMs for Hallucination Mitigation
Source: arXiv:2503.08216 source file (2025-03-14)
Supplement: Supplementary file 7 [file Appendix_MMVet.tex]

\begin{table}[h!]
\centering
\small
\resizebox{0.5 \linewidth}{!}{
\begin{tabular}{ll}
\toprule
\textbf{Method} & \textbf{Total} \\
\midrule
 LLaVA1.5-7B & 31.1 \basex{0.0} \\
  + VCD~\citep{leng2023mitigating_vcd} & 30.20 \downbad{0.9} \\
  + OPERA~\citep{huang2023opera} & 32 \up{0.9} \\
  \textbf{+ AID (Ours)} & \textbf{32.4} \up{1.3} \\ 
\midrule
 Qwen-VL-Chat & 49.0 \basex{0.0} \\
  + VCD~\citep{leng2023mitigating_vcd} & 34.60 \downbad{14.4} \\
  + OPERA~\citep{huang2023opera} & - \\
  \textbf{+ AID (Ours)} & \textbf{49.6} \up{0.6} \\
\midrule 
 GLM-4V-9B & 63.4 \basex{0.0} \\
   + VCD~\citep{leng2023mitigating_vcd} & 59.40 \downbad{4.0} \\
   + OPERA~\citep{huang2023opera} & - \\
   \textbf{+ AID (Ours)} & \textbf{65.0} \up{1.6} \\
\bottomrule
\end{tabular}}
\vspace{-5pt}
\caption{Results on MM-Vet dataset. Best-performing method per model size and dataset is highlighted in bold; arrows indicate improvement or degradation over the baseline, where lower values indicate better performance.}
\label{tab:res_mmvet}
\end{table}
