# Supplementary material for: Attention Hijackers: Detect and Disentangle Attention Hijacking in LVLMs for Hallucination Mitigation
Source: arXiv:2503.08216 source file (2025-03-14)
Supplement: Supplementary file 8 [file Appendix_Vizwiz.tex]

\begin{table}[t!]
\centering
\small
\resizebox{0.5 \linewidth}{!}{
\begin{tabular}{ll}
\toprule
\textbf{Method} & \textbf{Accuracy} \\
\midrule
 LLaVA1.5-7B & 50.00 \basex{0.0} \\
  + VCD~\citep{vcd2024cvpr} & 44.90 \downbad{5.1} \\
  + OPERA~\citep{opera2024cvpr} & 50.76 \up{0.8} \\
  \textbf{+ AID (Ours)} & \textbf{51.50} \up{1.5} \\ 
\midrule
 Qwen-VL-Chat & 66.05 \basex{0.0} \\
  + VCD~\citep{vcd2024cvpr} & 34.54 \downbad{31.5} \\
  + OPERA~\citep{opera2024cvpr} & - \\
  \textbf{+ AID (Ours)} & \textbf{66.36} \up{0.3} \\
\midrule 
 GLM-4V-9B & 57.39 \basex{0.0} \\
   + VCD~\citep{vcd2024cvpr} & 48.04 \downbad{9.4} \\
   + OPERA~\citep{opera2024cvpr} & - \\
   \textbf{+ AID (Ours)} & \textbf{58.00} \up{0.6} \\
\bottomrule
\end{tabular}}
\vspace{-5pt}
\caption{Results on Vizwiz dataset. Best-performing method per model size and dataset is highlighted in bold; arrows indicate improvement or degradation over the baseline, where lower values indicate better performance.}
\label{tab:res_vizwiz}
\end{table}
